# Supplementary material for: Self-Supervised Learning for Monocular Depth Estimation from Aerial Imagery
Source: arXiv:2008.07246 source file (2020-08-17)
Supplement: Supplementary file 1 [file 08_appendix.tex]

\section*{APPENDIX (Optional)}\label{Asec:appendix}

Any additional supporting data may be appended, provided the paper does not exceed the limits given above.
